# Supplementary material for: Learning Factorized Multimodal Representations
Source: arXiv:1806.06176 source file (2019-05-14)
Supplement: Supplementary file 1 [file ab_supple.tex]

\newcolumntype{K}[1]{>{\centering\arraybackslash}p{#1}}
\definecolor{gg}{RGB}{45,190,45}

\begin{table}[t!]
\fontsize{7.5}{10}\selectfont
%\centering
\setlength\tabcolsep{1.1pt}
\begin{tabular}{l : *{5}{K{0.97cm}} : l : *{5}{K{0.97cm}}}
\Xhline{3\arrayrulewidth}
Dataset & \multicolumn{5}{c:}{\textbf{CMU-MOSI}} & Dataset & \multicolumn{5}{c}{\textbf{CMU-MOSI}} \\
Task & \multicolumn{5}{c:}{Sentiment} & Task & \multicolumn{5}{c}{Sentiment} \\
Metric  & A$^{2}$ & F1 & A$^{7}$ & MAE & Corr & Metric & A$^{2}$ & F1 & A$^{7}$ & MAE & Corr \\ 
\Xhline{0.5\arrayrulewidth}
EF MM    & & & & & & MARN MM   & & & & &  \\
EF \ds    & 75.1 & 74.6 & 33.5 & 1.02 & \textbf{0.639} & MARN \ds  & 74.8 & 74.8 & 30.6 & 1.05 & 0.617 \\
EF \threes   & 74.9 & 75.0 & 33.1 & 1.02 & 0.627 & MARN \threes & 74.9 & 75.0 & \textbf{33.1} & \textbf{1.02} & 0.627 \\
EF GDDM    & & & & & & MARN GDDM   & & & & &  \\
EF \ones   & 74.8 & 74.7 & \textbf{33.7} & 1.03 & 0.627 & MARN \ones & 72.3 & 72.4 & 26.4 & 1.10 & 0.596 \\
EF \ours   & \textbf{75.2} & \textbf{75.3} & 32.8 & \textbf{1.02} & 0.629 & MARN \ours & \textbf{75.5} & \textbf{75.4} & 31.2 & 1.05 & \textbf{0.640} \\
\Xhline{0.5\arrayrulewidth}
TF MM    & & & & & & MFN MM   & 74.6 & 74.7 & 28.7 & 1.024 & 0.626 \\
TF \ds    & 75.1 & 75.1 & 27.0 & 1.10 & 0.643 & MFN \ds   & 76.1 & 76.0 & 28.7 & 1.043 & 0.634 \\
TF \threes   & 74.9 & 75.0 & \textbf{33.1} & \textbf{1.02} & 0.627 & MFN \threes & 74.9 & 75.0 & 33.1 & 1.023 & 0.627 \\
TF GDDM    & & & & & & MFN GDDM   & 74.3 & 74.4 & 31.9 & 1.039 & 0.610 \\
TF \ones   & 74.2 & 74.3 & 29.6 & 1.05 & 0.620 & MFN \ones  & 76.5 & 76.5 & 31.9 & 1.071 & 0.647 \\
TF \ours   & \textbf{75.5} & \textbf{75.4} & 30.9 & 1.05 & \textbf{0.648} & MFN \ours  & \textbf{77.3} & \textbf{77.2} & \textbf{35.4} & \textbf{0.961} & \textbf{0.661} \\
\Xhline{3\arrayrulewidth}
\end{tabular}
\caption{Sentiment prediction results on CMU-MOSI test set for comparing the performance of \ours \ with ablation baselines. Best scores per fusion model are indicated in bold. \ours \ generally achieves better results as compared to ablation baselines that remove disentangled and generative capabilities. A$^C$ = multiclass accuracy across $C$ classes, MAE = Mean Absolute Error, $r$ = Pearson's correlation.}
\label{ab_supple}
\end{table}
